# Supplementary material for: Evaluating Multi-label Classifiers with Noisy Labels
Source: arXiv:2102.08427 source file (2021-02-16)
Supplement: Supplementary file 1 [file supp.tex]

\section{Supplementary Material}
\subsection{Dataset Statistics}
\begin{table*}[t]
\centering
\resizebox{\textwidth}{!}{%
\begin{tabular}{l|llllllllllll}
Dataset    & Input Type    & \#Train & \#Val  & \#Test & Labels (L) & Features         & \begin{tabular}[c]{@{}l@{}}Mean\\ Label\\ /Sample\end{tabular} & \begin{tabular}[c]{@{}l@{}}Median\\ Label\\ /Sample\end{tabular} & \begin{tabular}[c]{@{}l@{}}Max\\ Label\\ /Sample\end{tabular} & \begin{tabular}[c]{@{}l@{}}Mean\\ Sample\\ /Label\end{tabular} & \begin{tabular}[c]{@{}l@{}}Median\\ Label\\ /Sample\end{tabular} & \begin{tabular}[c]{@{}l@{}}Max\\ Label\\ /Sample\end{tabular} \\ \hline
reuters    & Sequential    & 6,993   & 777    & 3,019  & 90         & 23662            & 1.23                                                           & 1                                                                & 15                                                            & 106.50                                                         & 18                                                               & 2,877                                                         \\
rcv1       & Sequential    & 703,135 & 78,126 & 23,149 & 103        & 368,998          & 3.21                                                           & 3                                                                & 17                                                            & 24,362                                                         & 7,250                                                            & 363,991                                                       \\
bibtex     & Binary Vector & 4,377   & 487    & 2515   & 159        & 1836             & 2.38                                                           & 2                                                                & 28                                                            & 72.79                                                          & 54                                                               & 689                                                           \\
delicious  & Binary Vector & 11,579  & 1,289  & 3,185  & 983        & 500              & 19.06                                                          & 20                                                               & 25                                                            & 250.15                                                         & 85                                                               & 5,189                                                         \\
Pascal VOC & Image         & 5011    & N/A    & 4952   & 20         & 448 $\times$ 448 & 1.56                                                           & 1                                                                & 7                                                             & 395.65                                                         & 268                                                              & 2,095                                                        
\end{tabular}%
}
\caption{\textbf{Dataset Statistics}. We select five datasets that vary in a number of aspects including the input type, number of samples, number of labels, and how imbalanced the label classes are.}
\label{tab:dataset_stats}
\end{table*}
We use five well-studied MLC datasets.
We show the dataset statistics in Table~\ref{tab:dataset_stats}: the five datasets vary in the input type, number of samples, number of labels, and number of input features; additionally, some datasets have more imbalanced classes than the others.

\subsection{Evaluation Metrics}
We use the following metrics in the experimental evaluation.
\paragraph{F1-scores.}
We denote the number of true positives by $tp$, the number of false positives by $fp$, and the number of false negatives by $fn$. An F1-score is defined as follows:
\begin{equation*}
    F_1 = \frac{2tp}{2tp+(fp+fn)}
\end{equation*}

The example-based F1-score calculates F1-scores for all test samples individually and take the average over them: 
\begin{equation*}
    \mathrm{eb}F_1=\frac{1}{N}\sum_{i=1}^{N}\frac{\sum_{j=1}^L 2y_j^i\hat{y}_j^i}{\sum_{j=1}^L y_j^i+\sum_{j=1}^L\hat{y}_j^i}
\end{equation*}
where $N$ is the number of test samples, $y_j^i$ is the $j$-th ground-truth label of test sample $i$ and $\hat{y}_j^i$ is the $j$-th predicted label of test sample $i$.

The micro-averaged F1-score sums up individual true positives, false positives, and false negatives of all predication outcomes, and use them to compute an F1-score: 
\begin{equation*}
    \mathrm{mi}F_1=\frac{\sum_{l=1}^L\sum_{i=1}^{N} 2y_l^i\hat{y}_l^i}{\sum_{l=1}^L\sum_{i=1}^{N}[2y_l^i\hat{y}_l^i+(1-y_l^i)\hat{y}_l^i+y_l^i(1-\hat{y}_l^i)]}
\end{equation*}
The macro-averaged F1-score is the averaged F1-score over all label classes: 
\begin{equation*}
   \mathrm{ma}F_1=\frac{1}{L}\sum_{l=1}^{L}\frac{ \sum_{i=1}^{N}2y_l^i\hat{y}_l^i}{\sum_{i=1}^{N} [2y_l^i\hat{y}_l^i+(1-y_l^i)\hat{y}_l^i+y_l^i(1-\hat{y}_l^i)]} 
\end{equation*}
\subsection{Additional Experiments}
\begin{figure*}[t]
    \centering
    \includegraphics[width=0.75\textwidth]{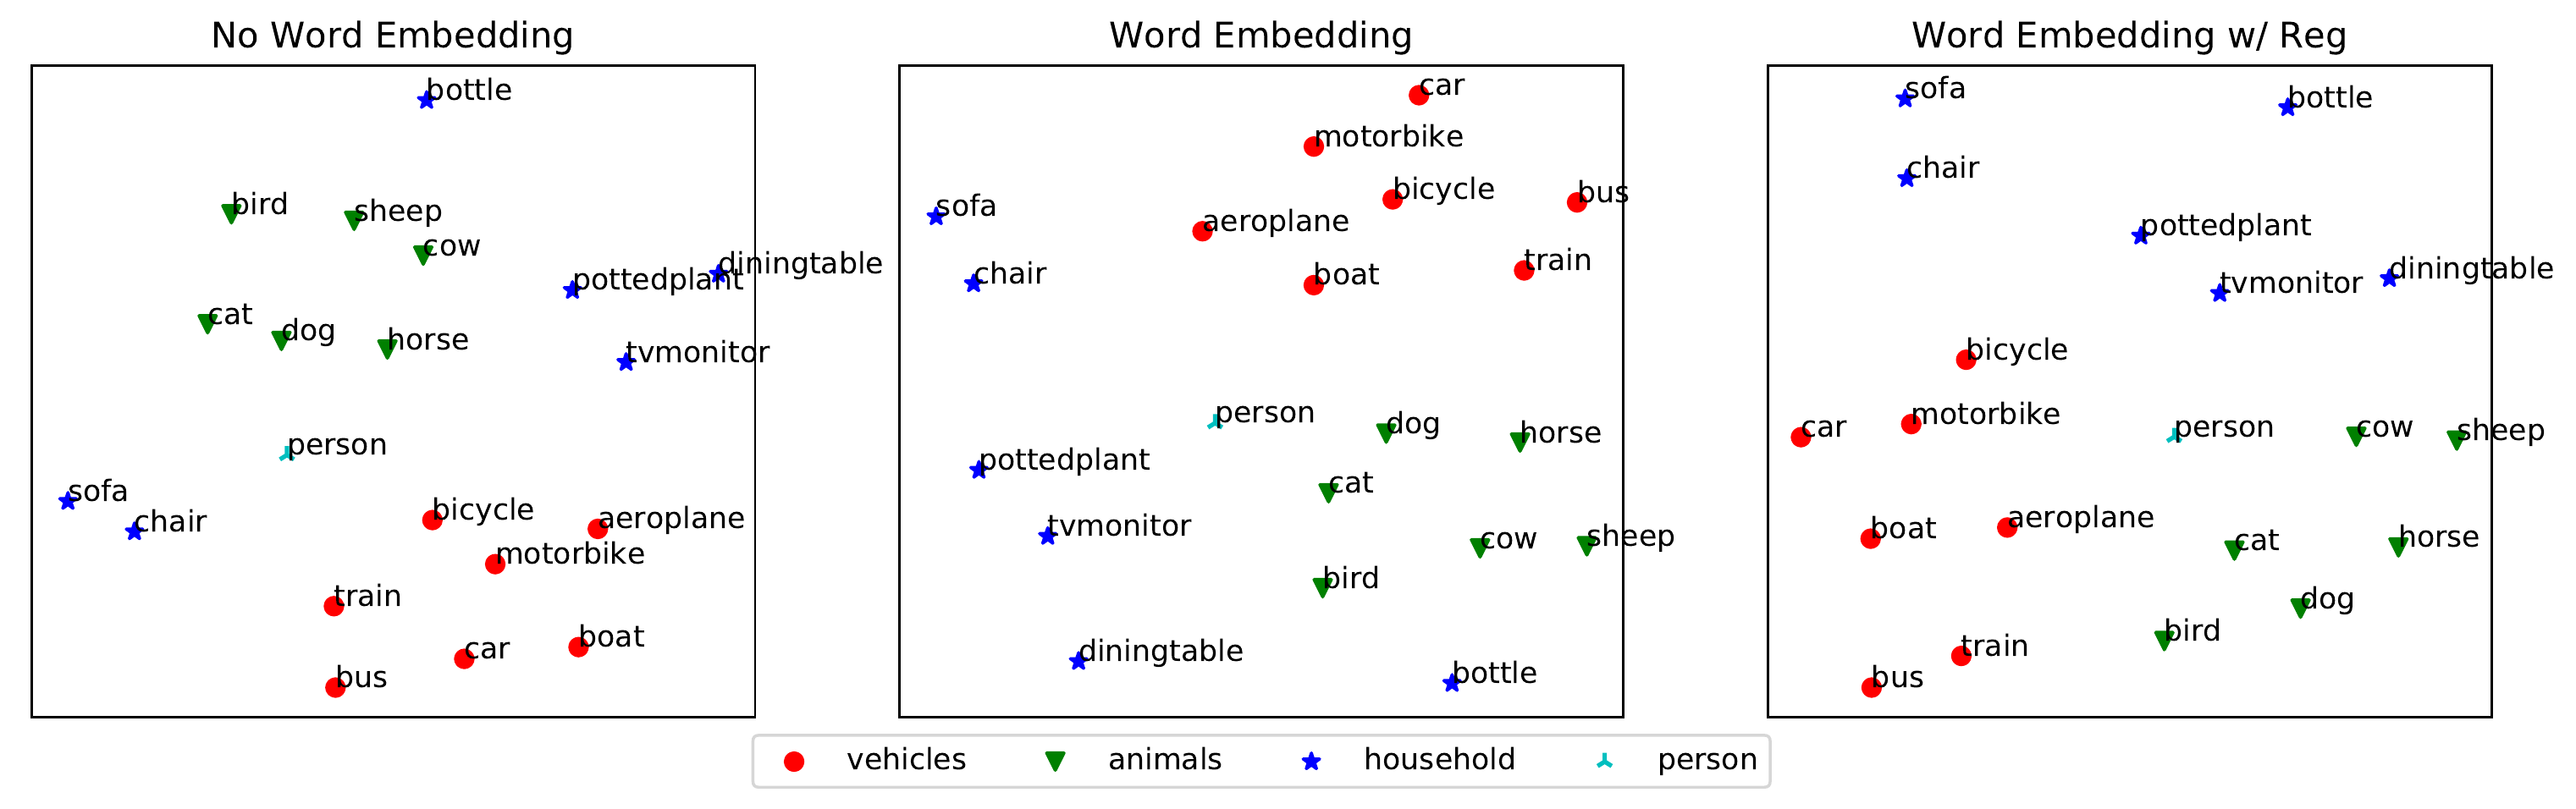}
    \caption{t-SNE visualization of various label embeddings on Pascal VOC. \textbf{Left:} Randomly initialized label embeddings learned over the training process. \textbf{Middle:} Fixed word embeddings as label embeddings. \textbf{Right:} Label embeddings initialized as word embeddings and learned with context-based regularization during training. \textit{While the first setting already produces label embeddings with good qualities, the last setting learns ``perfect'' label clusters.}}
    \label{fig:voc_tsne}
\end{figure*}
\subsubsection{Visualization} % embedding at the beginning, at the end
In Figure~\ref{fig:voc_tsne}, we present a t-SNE visualization~\cite{van2008visualizing} of label embeddings of \emph{Pascal VOC} obtained from various settings.
With enough training data, starting to learn with randomly initialized label embeddings already produces reasonable results.
However, with word embeddings, we are able to obtain more precise label clusterings.
The word embedding clusterings (middle) and the regularized word embedding clusterings (right) look similar.
That said, regularized word embeddings clusterings are more accurate in the context of \emph{Pascal VOC}; they begin from the word embeddings, but become more relevant to the dataset  through the training process.
Since the objects falling into the same category have more co-occurrences, they are closer to each other in the embedding space.

\subsubsection{When CbMLC fails}
\begin{table}[h]
\centering
\resizebox{0.45\textwidth}{!}{%
\begin{tabular}{c"c|c|c|c}
\multicolumn{1}{l}{} & \textbf{No WordEmb}            & \textbf{WordEmb 0.01} & \textbf{WordEmb 0.10} & \textbf{WordEmb 1.00} \\ \thickhline
\textbf{miF1}        & {\ul \textit{\textbf{0.4119}}} & 0.4117                & 0.4106                & 0.4104                \\
\textbf{maF1}        & {\ul \textit{\textbf{0.2538}}} & 0.238                 & 0.2375                & 0.2354               
\end{tabular}%
}
\caption{Performance comparison of using randomly initialized label embeddings to using label embbedings with context-based regularization on the \emph{ebird} dataset. The numbers next to WordEmb are the regularization coefficients. Highlighted numbers are the best of a row.}
\label{tab:ebird}
\end{table}

We briefly discuss when context-based regularization fails.
CbMLC is highly dependent on the quality of pretrained word embeddings.
We run it on an additional dataset, \emph{ebird}~\cite{sullivan2009ebird}, which is a bird distribution dataset across the world.
Given a set of environmental features $\bm{x}$ associated to a location, the task is to predict what bird species $\bm{y}$ there are at the given location.
Again, we retrieve species names from GloVe.
We summarize the results in Table~\ref{tab:ebird}.
Since these are less frequent words, initializing label embeddings as word embeddings yields a worst result than learning label embeddings from scratch.

\subsubsection{Comparing to a SOTA Single-Label Denoise Method}
While there is no regularization-based unsupervised method developed for noisy single-label learning that can be directly applied to MLC, we modify \emph{MD-DYR-SH}~\cite{arazo2019unsupervised} so that we can see how a SOTA single-label denoise method performs compared to CbMLC.
MD-DYR-SH is based on \emph{mixup}~\cite{zhang2018mixup}, which assumes inputs to be real numbers.
For this reason, MD-DYR-SH can only be applied on \emph{Pascal VOC}.

\begin{table}[t]
\centering
\resizebox{0.3\textwidth}{!}{%
\begin{tabular}{c"c|c|c}
\textbf{F1-score} & \textbf{MD-DYR-SH} & \textbf{ML-GCN} & \textbf{CbMLC}                 \\\thickhline
\textbf{miF1}     & 0.7290             & 0.7138          & {\ul \textit{\textbf{0.7621}}} \\
\textbf{maF1}     & 0.6396             & 0.6281          & {\ul \textit{\textbf{0.7281}}}
\end{tabular}%
}
\caption{Comparison of CbMLC to ML-GCN, a SOTA multi-label image recognition method, and MD-DYR-SH, a SOTA single-label denoise method. Highlighted numbers are the best of a row.}
\label{tab:single-label}
\end{table}

MD-DYR-SH leverages an observation that a deep model fits clean labels before noisy labels: they fit training loss curve with a beta mixture models (BMM) to identify noisy labels.
To adapt it for MLC, instead of only penalizing false negatives, we also add loss for false positives.
We test MD-DYR-SH with the combined noise.
We fine tune MD-DYR-SH to achieve its best possible performance and show the results in Table~\ref{tab:single-label}.
We can see that although, modified MD-DYR-SH slightly improves over ML-GCN, a SOTA multi-label image recognition method, the gap between MD-DYR-SH and CbMLC is still large.
Our intepretation is that single-label learning only optimizes on the one true positive label per instance, but the MLC loss simultaneously penalizes all misclassified labels for an instance; therefore, we need to develop regularization techniques that is suitable for the MLC loss rather than simply adapting approaches from single-label learning.

\subsubsection{Complete Results for Type 1 and Type 2 Noise}
\begin{table*}[h]
\centering
\resizebox{0.7\textwidth}{!}{%
\begin{tabular}{c|c"cc|cc|cc|cc|cc}
\multicolumn{2}{c}{\textbf{Noise Level}}              & \multicolumn{2}{c}{\textbf{0.01}}                               & \multicolumn{2}{c}{\textbf{0.02}}                               & \multicolumn{2}{c}{\textbf{0.03}}                               & \multicolumn{2}{c}{\textbf{0.04}}                               & \multicolumn{2}{c}{\textbf{0.05}}                               \\ \hline
\textbf{Dataset}                    & \textbf{Method} & \textbf{miF1}                  & \textbf{maF1}                  & \textbf{miF1}                  & \textbf{maF1}                  & \textbf{miF1}                  & \textbf{maF1}                  & \textbf{miF1}                  & \textbf{maF1}                  & \textbf{miF1}                  & \textbf{maF1}                  \\ \thickhline
\multirow{2}{*}{\textbf{delicious}} & \textbf{SOTA}   & {\ul \textit{\textbf{0.3794}}} & {\ul \textit{\textbf{0.1734}}} & {\ul \textit{\textbf{0.3732}}} & {\ul \textit{\textbf{0.1605}}} & {\ul \textit{\textbf{0.3677}}} & {\ul \textit{\textbf{0.1532}}} & {\ul \textit{\textbf{0.3612}}} & {\ul \textit{\textbf{0.1476}}} & {\ul \textit{\textbf{0.3452}}} & 0.1352                         \\
                                    & \textbf{CbMLC}  & 0.3668                         & 0.1409                         & 0.3544                         & 0.1409                         & 0.3543                         & 0.1409                         & 0.3482                         & 0.1409                         & 0.3306                         & {\ul \textit{\textbf{0.1409}}} \\
\multirow{2}{*}{\textbf{rcv1}}      & \textbf{SOTA}   & 0.8720                         & 0.7265                         & {\ul \textit{\textbf{0.8857}}} & 0.7232                         & {\ul \textit{\textbf{0.8704}}} & 0.7123                         & 0.8704                         & 0.7021                         & {\ul \textit{\textbf{0.8721}}} & 0.7158                         \\
                                    & \textbf{CbMLC}  & {\ul \textit{\textbf{0.8725}}} & {\ul \textit{\textbf{0.7372}}} & 0.8726                         & {\ul \textit{\textbf{0.7249}}} & 0.8688                         & {\ul \textit{\textbf{0.7242}}} & {\ul \textit{\textbf{0.8706}}} & {\ul \textit{\textbf{0.7212}}} & 0.8689                         & {\ul \textit{\textbf{0.7236}}}
\end{tabular}%
}
\caption{Performance comparison of CbMLC to the best SOTA model on the additional two datasets with type 1 noise. Higher scores are better. Highlighted numbers are the best of in each row.}
\label{tab:adduniform}
\end{table*}

\begin{table*}[h]
\centering
\resizebox{0.7\textwidth}{!}{%
\begin{tabular}{c|c"cc|cc|cc|cc|cc}
\multicolumn{2}{c}{\textbf{Noise Level}}              & \multicolumn{2}{c}{\textbf{0.1}}                               & \multicolumn{2}{c}{\textbf{0.2}}                               & \multicolumn{2}{c}{\textbf{0.3}}                               & \multicolumn{2}{c}{\textbf{0.4}}                               & \multicolumn{2}{c}{\textbf{0.5}}                               \\ \hline
\textbf{Dataset}                    & \textbf{Method} & \textbf{miF1}                  & \textbf{maF1}                  & \textbf{miF1}                  & \textbf{maF1}                  & \textbf{miF1}                  & \textbf{maF1}                  & \textbf{miF1}                  & \textbf{maF1}                  & \textbf{miF1}                  & \textbf{maF1}                  \\ \thickhline
\multirow{2}{*}{\textbf{delicious}} & \textbf{SOTA}   & {\ul \textit{\textbf{0.3689}}} & 0.1871                         & {\ul \textit{\textbf{0.3646}}} & 0.1867                         & {\ul \textit{\textbf{0.3644}}} & 0.1784                         & {\ul \textit{\textbf{0.3634}}} & 0.1755                         & {\ul \textit{\textbf{0.3620}}} & 0.1652                         \\
                                    & \textbf{CbMLC}  & 0.3668                         & {\ul \textit{\textbf{0.1933}}} & 0.3544                         & {\ul \textit{\textbf{0.1911}}} & 0.3543                         & {\ul \textit{\textbf{0.1839}}} & 0.3482                         & {\ul \textit{\textbf{0.1763}}} & 0.3306                         & {\ul \textit{\textbf{0.1708}}} \\
\multirow{2}{*}{\textbf{rcv1}}      & \textbf{SOTA}   & 0.8711                         & {\ul \textit{\textbf{0.7374}}} & 0.8707                         & {\ul \textit{\textbf{0.7357}}} & 0.8648                         & 0.7147                         & 0.8630                         & 0.7163                         & 0.8647                         & 0.7166                         \\
                                    & \textbf{CbMLC}  & {\ul \textit{\textbf{0.8720}}} & 0.7430                         & {\ul \textit{\textbf{0.8710}}} & 0.7350                         & {\ul \textit{\textbf{0.8712}}} & {\ul \textit{\textbf{0.7355}}} & {\ul \textit{\textbf{0.8674}}} & {\ul \textit{\textbf{0.7393}}} & {\ul \textit{\textbf{0.8658}}} & {\ul \textit{\textbf{0.7290}}}
\end{tabular}%
}
\caption{Performance comparison of CbMLC to the best SOTA model on the additional two datasets with type 2 noise. Higher scores are better. Highlighted numbers are the best of in each row.}
\label{tab:adduniformpos}
\end{table*}

We add the performance comparison of CbMLC to the best SOTA model on \emph{delicious} and \emph{rcv1}.
We present the results for type 1 noise in Table~\ref{tab:adduniform} and the results for type 2 noise in Table~\ref{tab:adduniformpos}.
For type 1 noise, the best SOTA model outperforms CbMLC at the beginning on \emph{delicious}, and the performance gap shrinks as the noise becomes more severe.
For \emph{rcv1}, our method generally improves over the best SOTA model.
However, due to the large numbers of labels in these two datasets, the noise we injected is relatively small, and therefore CbMLC provides a limited improvement. 
%Since the best SOTA model outperforms CbMLC on the clean \emph{delicious} dataset, and the noise is too little when the noise level is 0.01 through 0.05,

For type 2 noise on \emph{delicious}, better maF1 scores from CbMLC indicate that we are better with handling imbalanced classes, and better miF1 scores from the best SOTA model suggests that it performs better for classes with frequent labels under this noisy setting.
For type 2 noise on \emph{rcv1}, again, our improvement is larger for classes with less frequent labels.
Further, we can also improve on miF1 scores when the noise becomes more severe.
